# Supplementary material for: Consistent Amortized Clustering via Generative Flow Networks
Source: arXiv:2502.19337 source file (2025-02-26)
Supplement: Supplementary file 2 [file proofs.tex]

\section{PROOFS?}
